# Supplementary material for: Class-Specific Explainability for Deep Time Series Classifiers
Source: arXiv:2210.05411 source file (2022-10-11)
Supplement: Supplementary file 1 [file supplementary.tex]

% \twocolumn[
% \centering
% \Large\textbf{Supplementary Materials for "Learning Saliency Maps to Explain Deep Time Series Classifiers"}]

% \hspace{5pt}
% \hskip 1in

% \textbf{Contents}
% \begin{enumerate}
%     \item Case Studies
%     \item Learning to Perturb Visualization
%     \item Experimental results of Recurrent Neural Network
% \end{enumerate}

% \setcounter{section}{0}

\section{RNN Experimental Results}\label{sec:rnn_results}

We evaluate PERT for each dataset in section \ref{sec:Data}. For each dataset, we pre-train one Recurrent Neural Network (RNN) to serve as the classifier in need of explanation. We compare our method to all state-of-the-art methods in section \ref{sec:comp_methods}. AUC-difference experimental result related to RNN is shown in the table \ref{tab:rnn_nte_auc_table}. In all cases, PERT significantly outperforms all other state-of-the-art methods, the confidence suppression game result is publicly-available at \texttt{http://www.hiddenforreview.com}.

\section{Case Studies}
\textsc{Blip dataset}: The 10-timestep synthetic dataset is designed by choice in order to intuitively verify the explanation provided to showcase the black-box model's pattern identification capabilities. For class 0, there are 6 different variations of blip in the first five timesteps. For class 1, there exists a single pattern i.e, a single blip in the first five time steps. In order to test the black-box-model's capability to ignore certain common patterns, both the classes have a single blip in last 5 timesteps. In this dataset there is no well-defined ground-truth for which time steps are truly the most important. To overcome this limitation, we design a simple synthetic dataset, where some timesteps are essential to classification success, while some timesteps are entirely irrelevant. Specifically, we create a balanced dataset with two classes and a total of X training time series. Examples from the \textit{Negative} class having ones are timesteps 2-4 and examples from the \textit{Positive} class having any random combination of ones and zeros between timesteps 2 and 4. Timesteps six and seven are always ones and all other timesteps are always zeros. This way, to predict the class label of a time series, all a classifier needs to look at is timesteps two, three, and four.

% \subsection{ \textbf{Blip Dataset}.}
\begin{figure}[htp]
% \hspace{-0.1 in}
 \centering
  \includegraphics[scale=0.033]{fig/blip_case.png}
  \caption{Blip Case Study. The signal is represented in Blue color and salient values are plotted against time steps. Important time steps are shown in green color for the class and in red color against the class with increasing brightness.}
%   \caption{\tnote{GIVE ME A CAPTION!}}
  \label{fig:CaseStudy}
\end{figure}

\section{Visualizing Perturbations: Sampled vs Learned}
% trim=left bottom right top, clip
% trim={0 1cm 4cm 4.5cm},clip
% \begin{align*}
\noindent
\hspace{-0.2 in}
\begin{minipage}{.3\textwidth}
  \centering
  \includegraphics[scale=.058, trim={0 1cm 4cm 4.5cm},clip]{fig/lime_perturbations.png}
  \captionof{figure}{LIME}
  \label{fig:LimePerturbations}
\end{minipage}
\hspace{-0.6 in}
\begin{minipage}{.3\textwidth}
  \centering
  \includegraphics[scale=.058, trim={0 1cm 11cm 3cm},clip]{fig/pert_perturbations.png}
  \captionof{figure}{PERT}
  \label{fig:TSPERTPerturbations}
\end{minipage}
% \end{align*}

\bigskip
Figures \ref{fig:LimePerturbations} and \ref{fig:TSPERTPerturbations} visualize perturbations from LIME \cite{Ribeiro2016WhySI} and PERT, reduced to \textit{two} dimensions by applying t-SNE.% \cite{Maaten2008VisualizingDU}.
 The color matches the perturbations and the bold black \textbf{``$\times$''} indicates the instance-of-interest $\hat{X}$. Figure \ref{fig:LimePerturbations} shows that the stochastic perturbations created by LIME are randomly selected surrounding $\hat{X}$, as expected. PERT, on the other hand, \textit{learns} to perturb $\hat{X}$, trace a path around $\hat{X}$.
This comparison clearly shows by example that LIME does not adapt its perturbations to $\hat{X}$. On the contrary, PERT's \textit{learned} perturbation function traces out a path unique to each instance, carefully developing an instance-specific explanation strategy.
